# Supplementary material for: G-NeuroDAVIS: A Neural Network model for generalized embedding, data visualization and sample generation
Source: arXiv:2410.14223 ancillary file (2024-10-18)
Supplement: Supplementary file 1 [file G_NeuroDAVIS_Supplementary.pdf]

# G-NeuroDAVIS: A model for generalized embedding, data visualization and sample generation

## Supplementary Material

Chayan Maitra, Rajat K. De\*

*Machine Intelligence Unit, Indian Statistical Institute, Kolkata, 203 Barrackpore Trunk Road, Kolkata 700108, India*

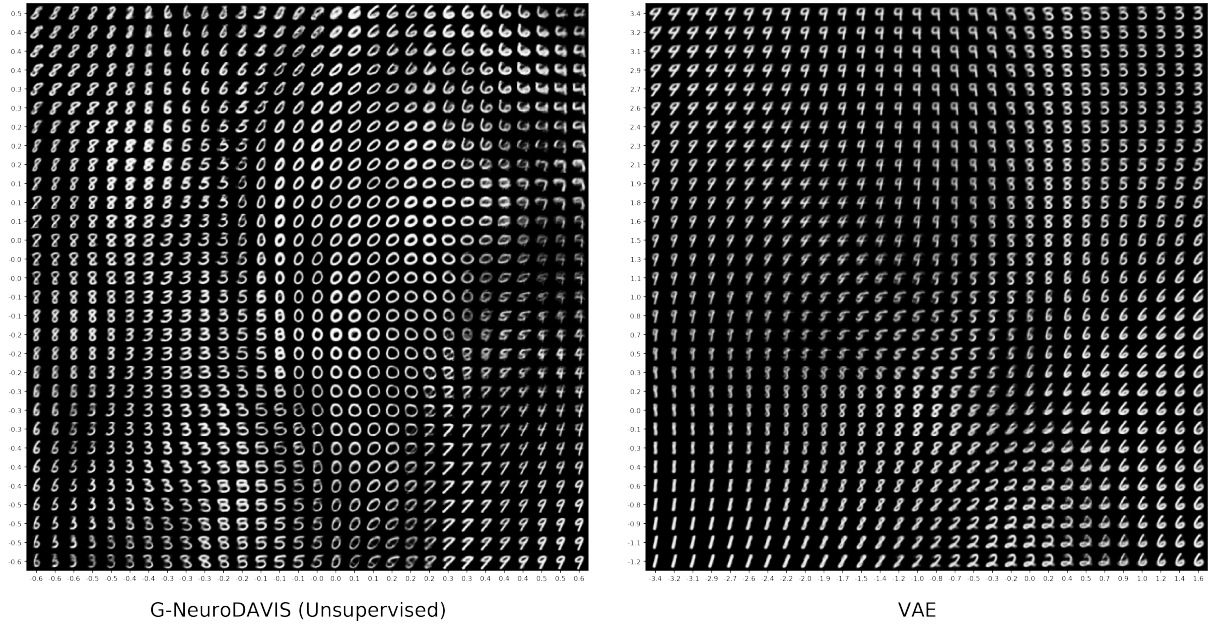

Figure S1: Mapping from 2-dimensional embedding, produced by G-NeuroDAVIS and VAE, in an unsupervised fashion, to the original high-dimensional space for *MNIST* dataset.

\*Corresponding author

Email addresses: [chayanmath25@gmail.com](mailto:chayanmath25@gmail.com) (Chayan Maitra), [rajat@isical.ac.in](mailto:rajat@isical.ac.in) (Rajat K. De)

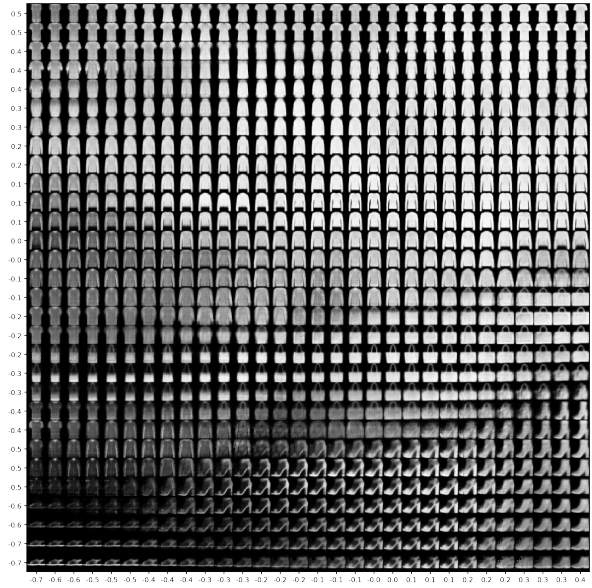

G-NeuroDAVIS (Unsupervised)

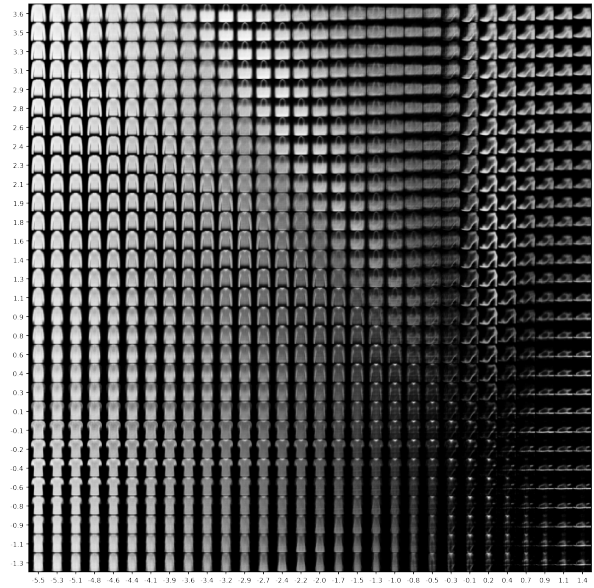

VAE

Figure S2: Mapping from 2-dimensional embedding, produced by VAE, to the original high-dimensional space for *FMNIST* dataset.

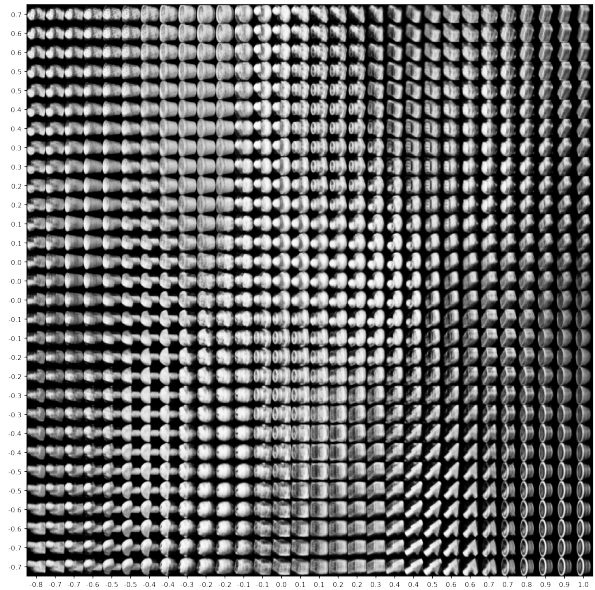

G-NeuroDAVIS (Unsupervised)

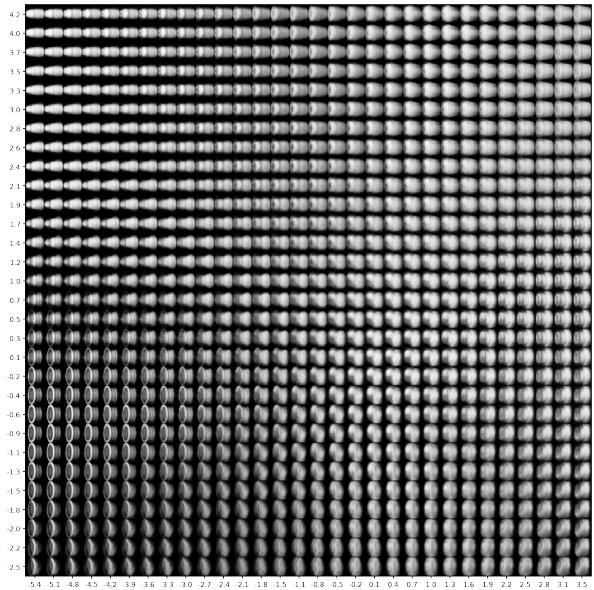

VAE

Figure S3: Mapping from 2-dimensional embedding, produced by G-NeuroDAVIS, in an unsupervised fashion, to the original high-dimensional space for *Coil20* dataset.

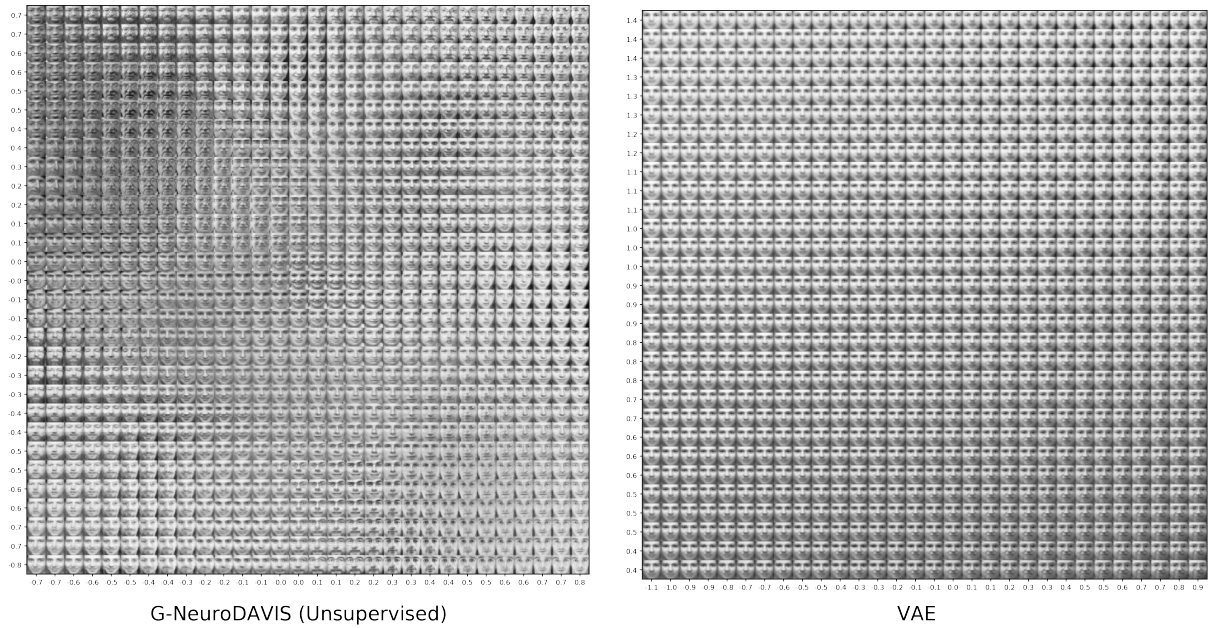

Figure S4: Mapping from 2-dimensional embedding, produced by G-NeuroDAVIS, in an unsupervised fashion, to the original high-dimensional space for *OlivettiFaces* dataset.

**A**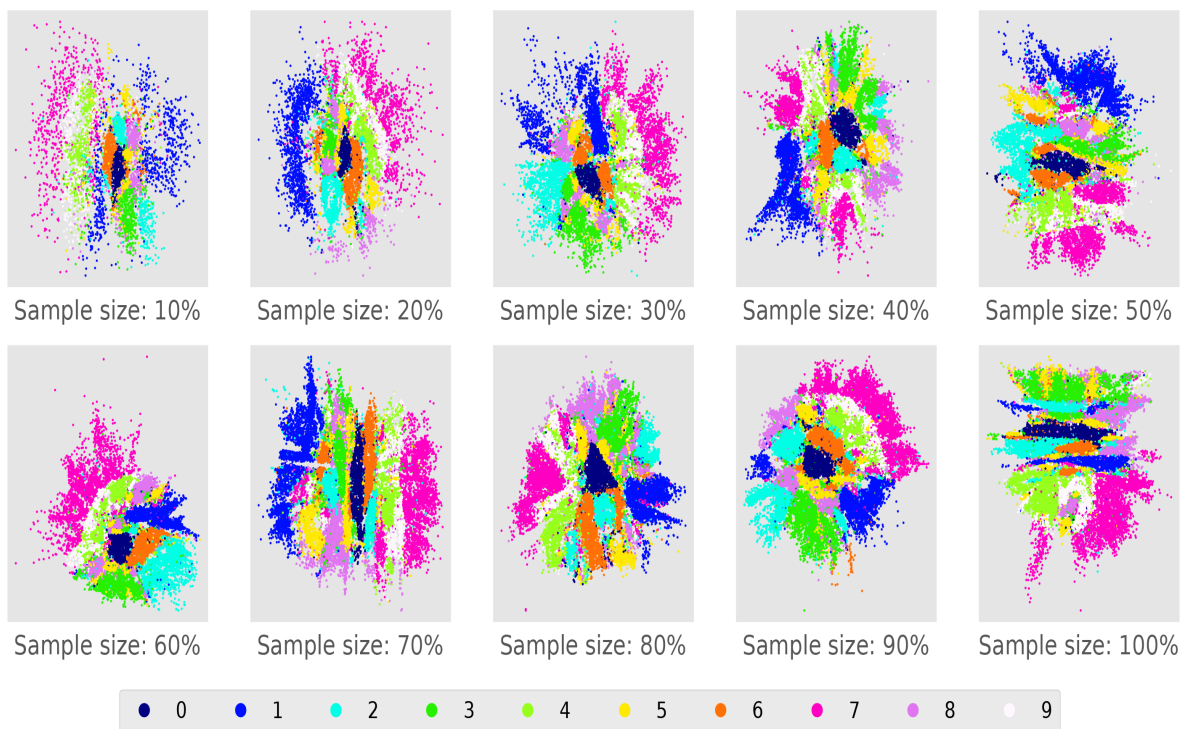**B**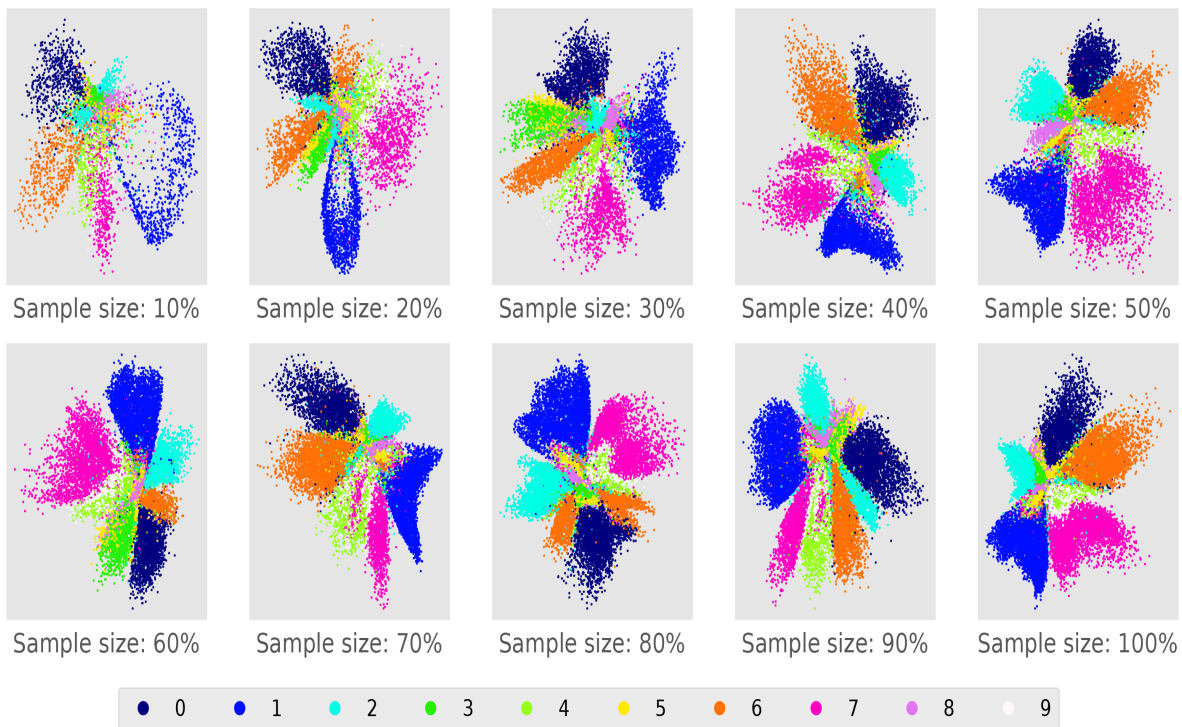

Figure S5: 2-dimensional embeddings produced by **(A)** G-NeuroDAVIS and **(B)** VAE, in an unsupervised fashion, for different sub-samples with varying sizes of *MNIST* dataset, coloured by different digits.

**A**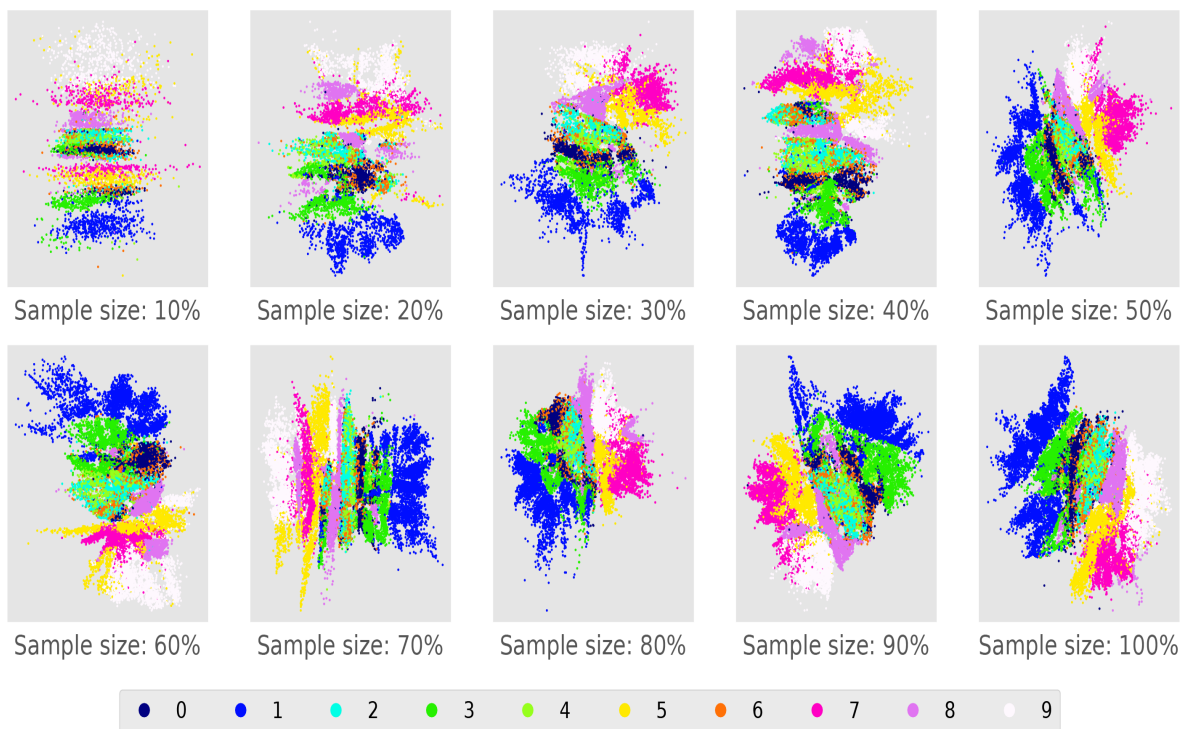**B**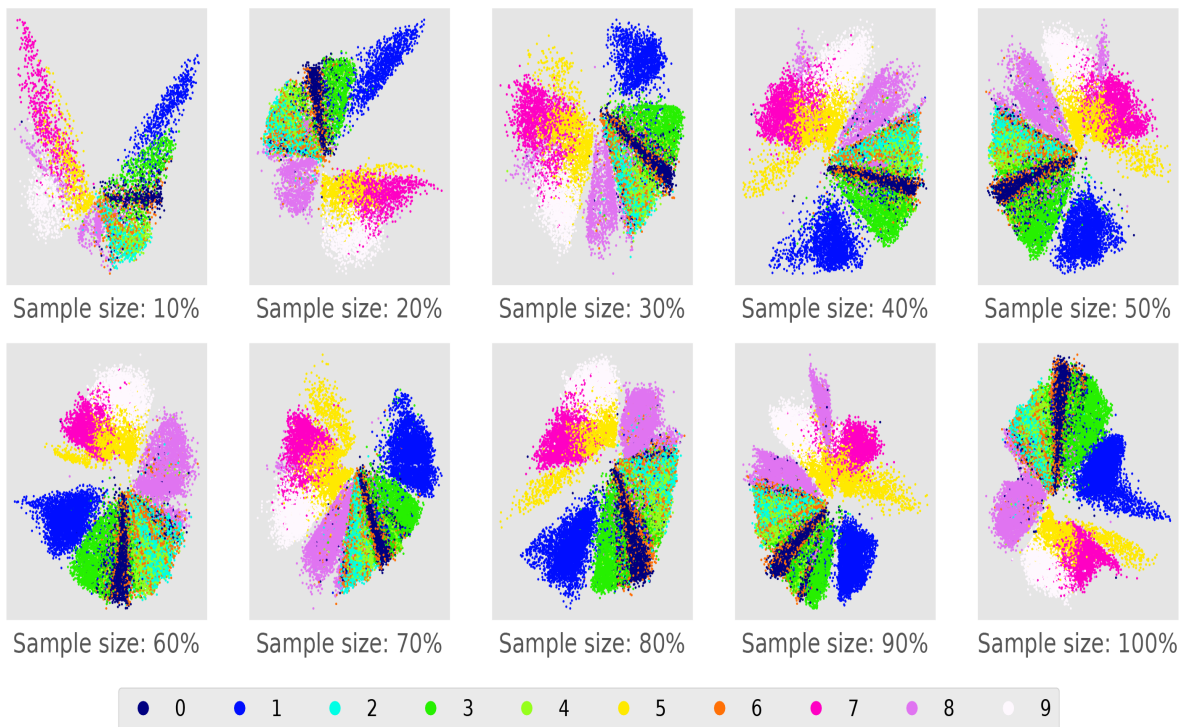

Figure S6: 2-dimensional embeddings produced by (A) G-NeuroDAVIS and (B) VAE, in an unsupervised fashion, for different sub-samples with varying sizes of *FMNIST* dataset, coloured by clothing's label.

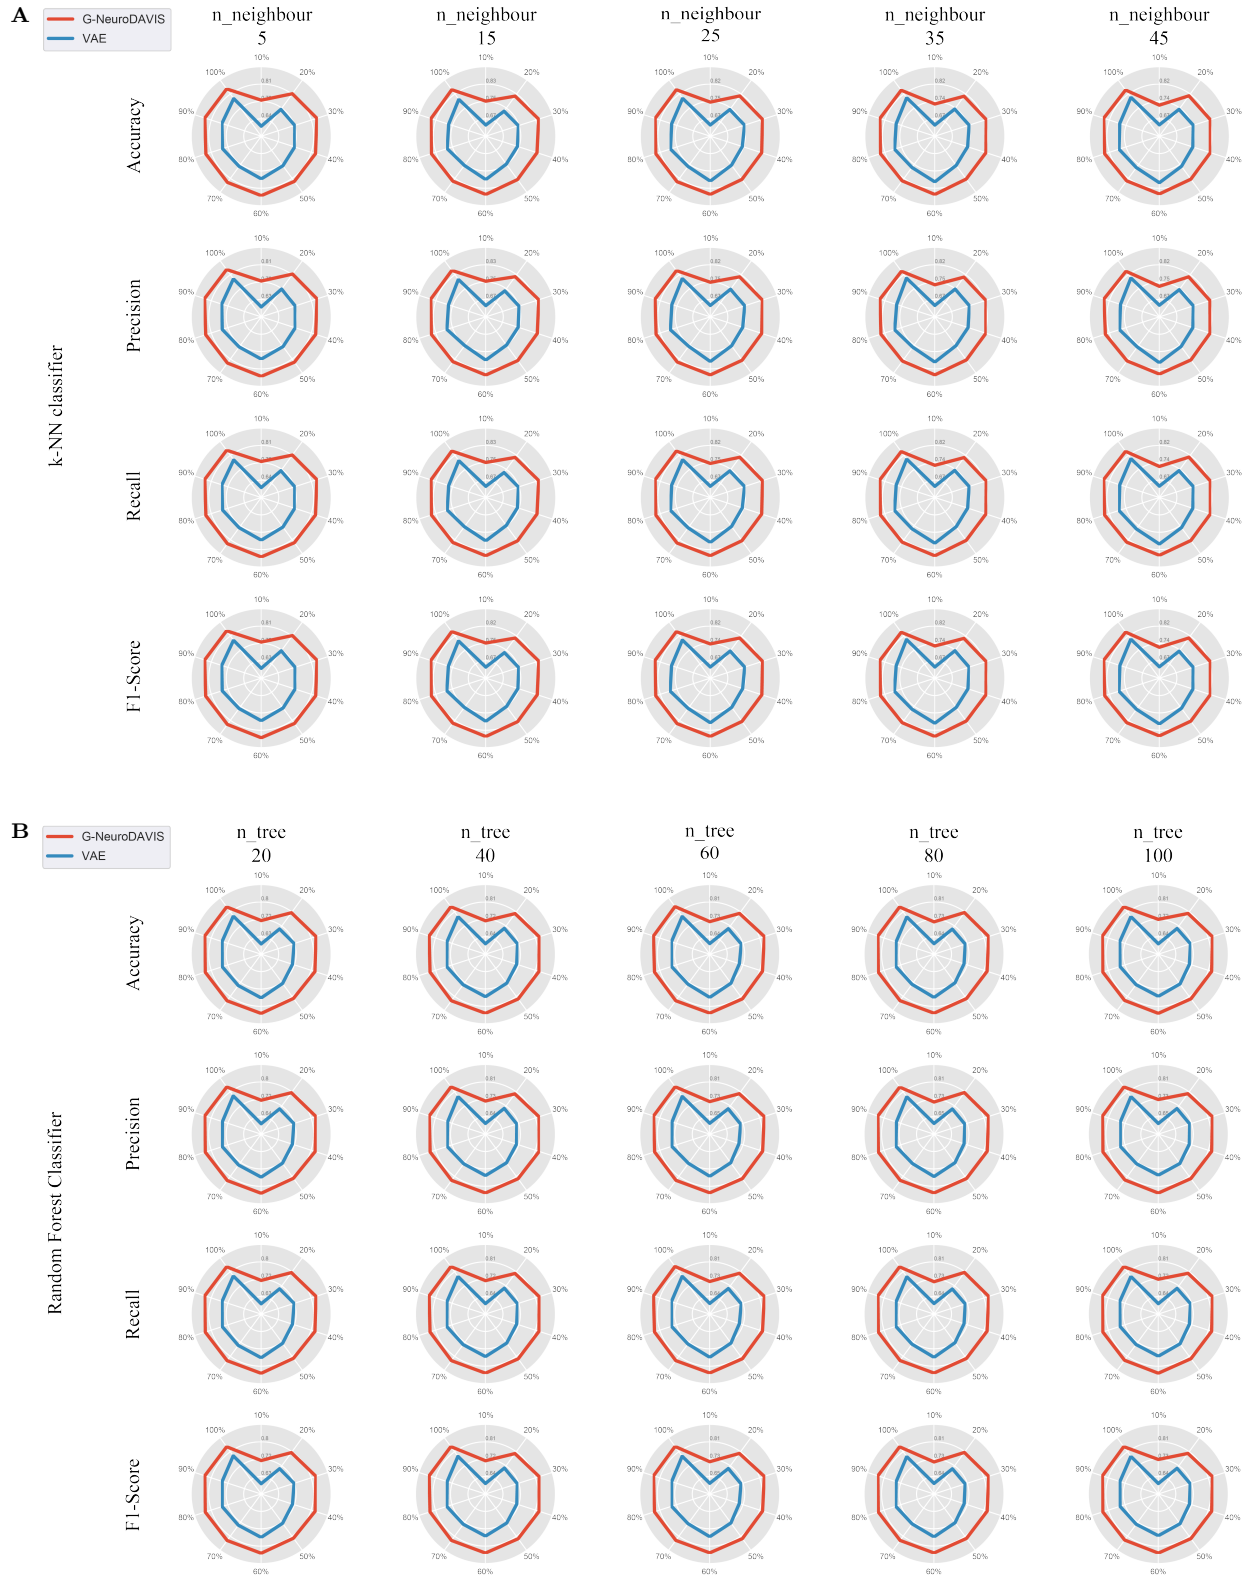

Figure S7: Classification performance of (A) k-NN and (B) RF on G-NeuroDAVIS-generated embedding against that obtained using VAE for different sub-samples with varying sizes of *MNIST* dataset in terms of Accuracy, Precision, Recall and F1-Score.

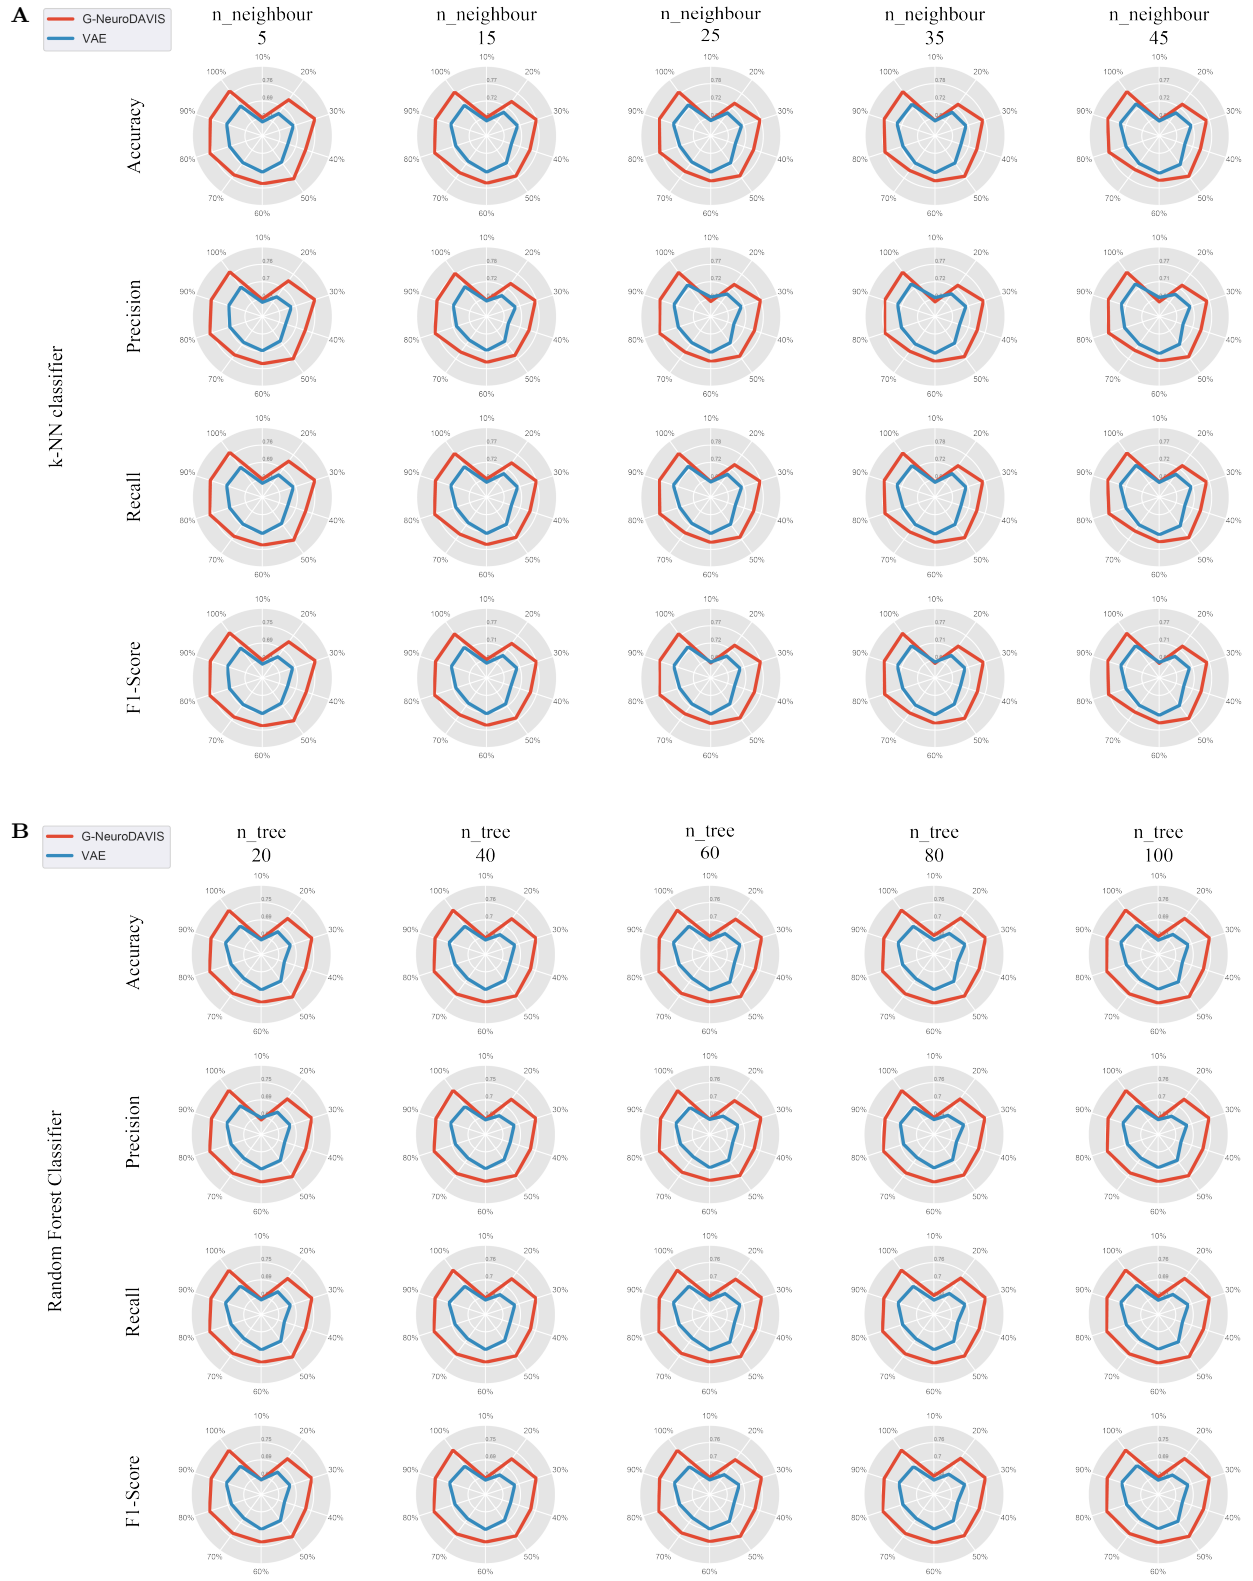

Figure S8: Classification performance of (A) k-NN and (B) RF on G-NeuroDAVIS-generated embedding against that obtained using VAE for different sub-samples with varying sizes of *FMNIST* dataset in terms of Accuracy, Precision, Recall and F1-Score.

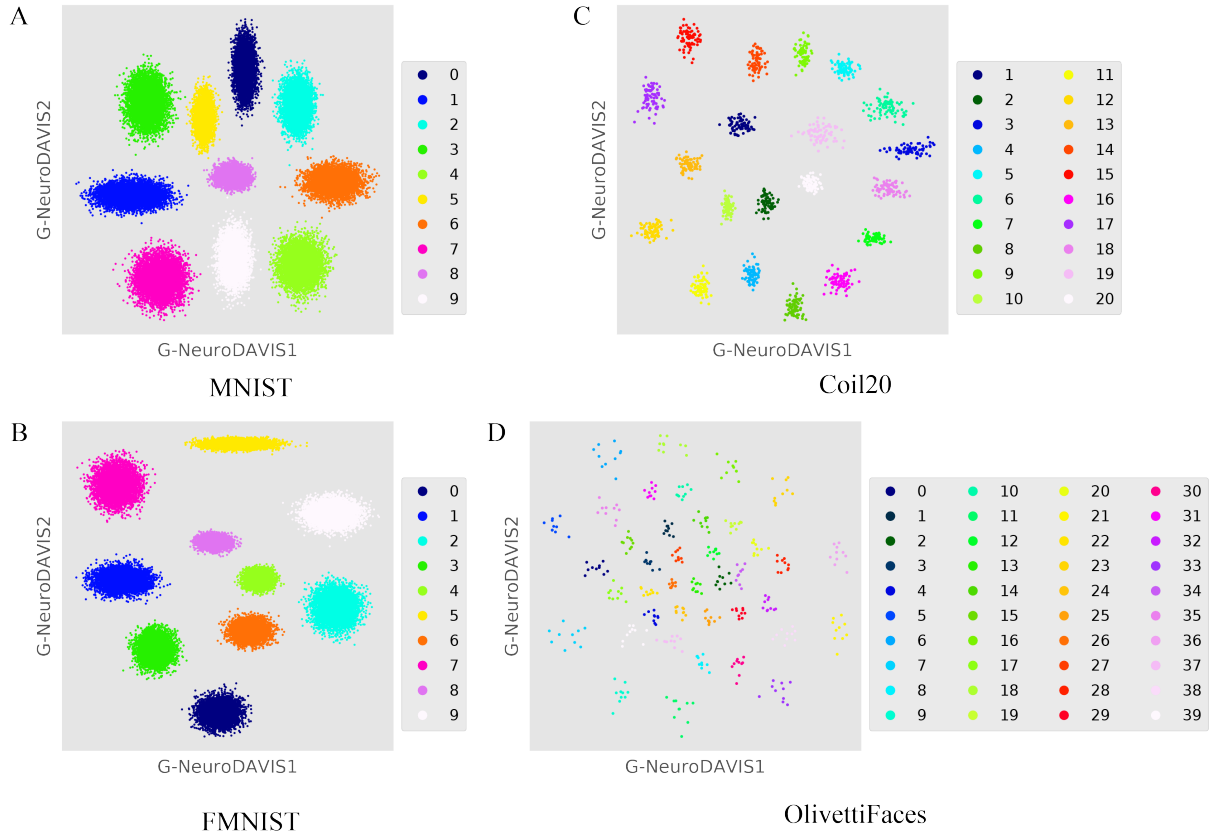

Figure S9: Embeddings produced by G-NeuroDAVIS, in an Supervised setting, for (A) *MNIST*, (B) *FMNIST*, (C) *Coil20* and (D) *OlivettiFaces* dataset
